# Supplementary material for: Bayesian inference for cluster-randomized trials with multivariate outcomes subject to both truncation by death and missingness
Source: arXiv:2505.02310 ancillary file (2025-05-05)
Supplement: Supplementary file 1 [file supp_Bivariate_Bayesian_SACE_Missing_Data__arxiv_Copy.pdf]

---

# Supplement materials for "Bayesian inference for cluster-randomized trials with multivariate outcomes subject to both truncation by death and missingness"

Guangyu Tong<sup>\*1,2,3,4</sup>, Chenxi Li<sup>5</sup>, Eric Velazquez<sup>1</sup>, Michael O. Harhay<sup>6,7</sup>, and Fan Li<sup>1,2,4</sup>

<sup>1</sup>Department of Internal Medicine, Section of Cardiovascular Medicine, Yale School of Medicine, New Haven, CT, USA

<sup>2</sup>Department of Biostatistics, Yale School of Public Health, New Haven, Connecticut, USA

<sup>3</sup>Cardiovascular Medicine Analytics Center, Yale School of Medicine, New Haven, Connecticut, USA

<sup>4</sup>Center for Methods in Implementation and Prevention Science, Yale University, New Haven, Connecticut, USA

<sup>5</sup>Department of Biostatistics & Bioinformatics, Duke School of Medicine, Durham, North Carolina, USA

<sup>6</sup>Clinical Trials Methods and Outcomes Lab, Palliative and Advanced Illness Research (PAIR) Center, Perelman School of Medicine, University of Pennsylvania, Philadelphia, Pennsylvania, USA

<sup>7</sup>Department of Biostatistics, Epidemiology and Informatics, Perelman School of Medicine, University of Pennsylvania, Philadelphia, Pennsylvania, USA

**\*Corresponding Author:** Guangyu Tong, PhD

**Email:** [guangyu.tong@yale.edu](mailto:guangyu.tong@yale.edu)

May 4, 2025

## Abstract

Cluster-randomized trials (CRTs) on fragile populations frequently encounter complex attrition problems where the reasons for missing outcomes can be heterogeneous, with participants who are known alive, known to have died, or with unknown survival status, and with complex and distinct missing data mechanisms for each group. Although existing methods have been developed to address death truncation in CRTs, no existing methods can jointly accommodate participants who drop out for reasons unrelated to mortality or serious illnesses, or those with an unknown survival status. This paper proposes a Bayesian framework for estimating survivor average causal effects in CRTs while accounting for different types of missingness. Our approach uses a multivariate outcome that jointly estimates the causal effects, and in the posterior estimates, we distinguish the individual-level and the cluster-level survivor average causal effect. We perform simulation studies to evaluate the performance of our model and found low bias and high coverage on key parameters across several different scenarios. We use data from a geriatric CRT to illustrate the use of our model. Although our illustration focuses on the case of a bivariate continuous outcome, our model is straightforwardly extended to accommodate more than two endpoints as well as other types of endpoints (e.g., binary). Thus, this work provides a general modeling framework for handling complex missingness in CRTs and can be applied to a wide range of settings with aging and palliative care populations.

**Keywords:** Bayesian inference, survivor individual-average causal effect, survivor cluster-average causal effect, informative cluster size, multivariate outcomes, nested missingness at random

## APPENDIX A: DETAILED DERIVATIONS FOR THE MARKOV CHAIN MONTE CARLO ALGORITHM

Following the prior distributions in Section 4.3, the posteriors can be derived as follows.

Step 1:

(1) For  $\alpha_{11,1}$ :

$$\begin{aligned}\alpha_{11,1} &\sim MVN(\mathbf{m}_{11,1}, \mathbf{v}_{11,1}) \\ \mathbf{v}_{11,1} &= \left[ \Sigma_e^{-1} \otimes \sum_{i=1}^n \sum_{j \in G_{11}} Z_i * \mathbf{X}_{ij} \mathbf{X}_{ij}^T + (\Sigma_{11,1})^{-1} \right]^{-1} \\ \mathbf{m}_{11,1} &= \mathbf{v}_{11,1} \left[ \Sigma_e^{-1} * \sum_{i=1}^n \sum_{j \in G_{11}} \begin{pmatrix} Z_i * \mathbf{X}_{ij} (y_{ij}^1 - \eta_i^1) \\ Z_i * \mathbf{X}_{ij} (y_{ij}^2 - \eta_i^2) \end{pmatrix} + (\Sigma_{11,1})^{-1} \alpha_{11,1} \right]\end{aligned}$$

(2) For  $\alpha_{11,0}$ :

$$\begin{aligned}\alpha_{11,0} &\sim MVN(\mathbf{m}_{11,0}, \mathbf{v}_{11,0}) \\ \mathbf{v}_{11,0} &= \left[ \Sigma_e^{-1} \otimes \sum_{i=1}^n \sum_{j \in G_{11}} (1 - Z_i) * \mathbf{X}_{ij} \mathbf{X}_{ij}^T + (\Sigma_{11,0})^{-1} \right]^{-1} \\ \mathbf{m}_{11,0} &= \mathbf{v}_{11,0} \left[ \Sigma_e^{-1} * \sum_{i=1}^n \sum_{j \in G_{11}} \begin{pmatrix} (1 - Z_i) * \mathbf{X}_{ij} (y_{ij}^1 - \eta_i^1) \\ (1 - Z_i) * \mathbf{X}_{ij} (y_{ij}^2 - \eta_i^2) \end{pmatrix} + (\Sigma_{11,0})^{-1} \alpha_{11,0} \right]\end{aligned}$$

(3) For  $\alpha_{10,1}$ :

$$\begin{aligned}\alpha_{10,1} &\sim MVN(\mathbf{m}_{10,1}, \mathbf{v}_{10,1}) \\ \mathbf{v}_{10,1} &= \left[ \Sigma_e^{-1} \otimes \sum_{i=1}^n \sum_{j \in G_{10}} Z_i * \mathbf{X}_{ij} \mathbf{X}_{ij}^T + (\Sigma_{10,1})^{-1} \right]^{-1} \\ \mathbf{m}_{10,1} &= \mathbf{v}_{10,1} \left[ \Sigma_e^{-1} * \sum_{i=1}^n \sum_{j \in G_{10}} \begin{pmatrix} Z_i * \mathbf{X}_{ij} (y_{ij}^1 - \eta_i^1) \\ Z_i * \mathbf{X}_{ij} (y_{ij}^2 - \eta_i^2) \end{pmatrix} + (\Sigma_{10,1})^{-1} \alpha_{10,1} \right]\end{aligned}$$

Step 2:

Let  $s_i$  be the number of individuals in the  $i$ th cluster that are alive. For  $\eta_i$ ,

$$\begin{aligned}\eta_i &\sim MVN(\mathbf{m}_{\eta_i}, \mathbf{v}_{\eta_i}) \\ \mathbf{v}_{\eta_i} &= [s_i * (\Sigma_e)^{-1} + (\Sigma_{\eta})^{-1}]^{-1} \\ \mathbf{m}_{\eta_i} &= \mathbf{v}_{\eta_i} (\Sigma_e)^{-1} \sum_{i=1}^s Z_i \left[ \sum_{j \in G_{11}} (\mathbf{y}_{ij} - \mathbf{X}_{ij}^T \alpha_{11,1}) + \sum_{j \in G_{10}} (\mathbf{y}_{ij} - \mathbf{X}_{ij}^T \alpha_{10,1}) \right] \\ &\quad + \mathbf{v}_{\eta_i} (\Sigma_e)^{-1} \sum_{i=1}^s (1 - Z_i) \left[ \sum_{j \in G_{11}} (\mathbf{y}_{ij} - \mathbf{X}_{ij}^T \alpha_{11,0}) \right]\end{aligned}$$

Step 3:

For  $\Sigma_{\eta}$ ,

$$\Sigma_{\eta} \sim IW(df = d^*, scale = (\mathbf{V}_{\eta}^*)^{-1})$$

$$d^* = d + n$$

$$\mathbf{V}_{\eta}^* = \mathbf{V}_{\eta} + \sum_{i=1}^n \eta_i \eta_i^T$$

Step 4:

Let  $N$  be the total number of individuals alive. For  $\Sigma_e$ ,

$$\Sigma_e \sim IW(df = d^*, scale = (V_e^*)^{-1})$$

$$d^* = d + n$$

$$V_e^* = V_e + \sum_{i=1}^n Z_i \left( \sum_{j \in G_{11}} (y_{ij} - X_{ij}^T \alpha_{11,1} - \eta_i)(y_{ij} - X_{ij}^T \alpha_{11,1} - \eta_i)^T + \sum_{j \in G_{10}} (y_{ij} - X_{ij}^T \alpha_{10,1} - \eta_i)(y_{ij} - X_{ij}^T \alpha_{10,1} - \eta_i)^T \right) \\ + \sum_{i=1}^n (1 - Z_i) \left( \sum_{j \in G_{11}} (y_{ij} - X_{ij}^T \alpha_{11,0} - \eta_i)(y_{ij} - X_{ij}^T \alpha_{11,0} - \eta_i)^T \right)$$

Step 5:

For  $\beta$ ,

$$\beta \sim (m_\beta, v_\beta)$$

$$v_\beta = \left[ \sum_{i=1}^n \sum_j X_{ij} X_{ij}^T + \Lambda^{-1} \right]^{-1}$$

$$m_\beta = v_\beta \left[ \sum_{i=1}^n \sum_j (Q_{ij} - \chi_i) X_{ij} + \Lambda^{-1} b \right]$$

Step 6:

For  $\gamma$ ,

$$\gamma \sim (m_\gamma, v_\gamma)$$

$$v_\gamma = \left[ (ij \in (G_{10}, G_{11})) \sum_{i=1}^n \sum_j X_{ij} X_{ij}^T + \Gamma^{-1} \right]^{-1}$$

$$m_\gamma = v_\gamma \left[ (ij \in (G_{10}, G_{11})) \sum_{i=1}^n \sum_j (W_{ij} - \chi_i) X_{ij} + \Gamma^{-1} r \right]$$

Step 7:

For  $\phi^2$ ,

$$\phi^2 \sim IG(shape = g + \frac{n}{2}, rate = h + \frac{1}{2} \sum_{i=1}^n \chi_i^2)$$

Step 8:

For  $\chi_i$ ,

$$\chi_i \sim \mathcal{N}(m_{\chi_i}, v_{\chi_i})$$

$$v_{\chi_i} = \left( m_i + \frac{1}{\phi^2} \right)^{-1}$$

$$m_{\chi_i} = v_{\chi_i} \left[ \sum_{j=1}^{n_i^*} (Q_{ij} - X_{ij}^T \beta) \right]$$

Step 9:

Update the strata membership of patients following the Bayes rule for subjects in Section 4.1,

(a) if  $D_i = 1$  and  $S_{ij}(1) = 0$ , then  $G_{ij} = 00$ .

(b) if  $D_i = 0$  and  $S_{ij}(0) = 1$ , then  $G_{ij} = 11$ .

(c) if  $D_i = 0$  and  $S_{ij}(0) = 0$ , then

$$P_{ij}(00) = \Psi(X_{ij}^T \beta + \chi_i)$$

$$P_{ij}(10) = (1 - \Psi(X_{ij}^T \beta + \chi_i)) * \Psi(X_{ij}^T \gamma + \chi_i)$$

$$M_{ij} \sim \text{Bernoulli} \left( \frac{P_{ij}(00)}{P_{ij}(00) + P_{ij}(10)} \right)$$

If  $M_{ij} = 1, G_{ij} = 00$ ; If  $M_{ij} = 0, G_{ij} = 10$ .

(d) if  $D_i = 1$  and  $S_{ij}(1) = 1$ , then

$$P_{ij}(10) = \Psi(\mathbf{X}_{ij}^T \boldsymbol{\gamma} + \chi_i) * p_{MVN}(\mathbf{Y}_{ij} - \mathbf{X}_{ij}^T \boldsymbol{\alpha}_{10,1} - \boldsymbol{\eta}_i, \boldsymbol{\Sigma}_e)$$

$$P_{ij}(11) = (1 - \Psi(\mathbf{X}_{ij}^T \boldsymbol{\gamma} + \chi_i)) * p_{MVN}(\mathbf{Y}_{ij} - \mathbf{X}_{ij}^T \boldsymbol{\alpha}_{11,1} - \boldsymbol{\eta}_i, \boldsymbol{\Sigma}_e)$$

$$M_{ij} \sim \text{Bernoulli}\left(\frac{P_{ij}(10)}{P_{ij}(10) + P_{ij}(11)}\right)$$

If  $M_{ij} = 1, G_{ij} = 10$ ; If  $M_{ij} = 0, G_{ij} = 11$ .

Step 10:

For each  $Q_{ij}$ , sample from the following truncated normal distributions,

$$Q_{ij} \sim \mathcal{N}_{Q_{ij} > 0}(\mathbf{X}_{ij}^T \boldsymbol{\beta} + \chi_i, 1), \text{ if } (G_{ij} = 00)$$

$$Q_{ij} \sim \mathcal{N}_{Q_{ij} \leq 0}(\mathbf{X}_{ij}^T \boldsymbol{\beta} + \chi_i, 1), \text{ if } (G_{ij} = 10|11)$$

Step 11:

For each  $W_{ij \in (G_{10}, G_{11})}$ , sample from the following truncated normal distributions,

$$W_{ij \in (G_{10}, G_{11})} \sim \mathcal{N}_{W_{ij} > 0}(\mathbf{X}_{ij}^T \boldsymbol{\gamma} + \chi_i, 1), \text{ if } (G_{ij} = 10)$$

$$W_{ij \in (G_{10}, G_{11})} \sim \mathcal{N}_{W_{ij} \leq 0}(\mathbf{X}_{ij}^T \boldsymbol{\gamma} + \chi_i, 1), \text{ if } (G_{ij} = 11)$$

## APPENDIX B: SIMULATION ACCESSING THE PERFORMANCE OF THE JOINT MODEL

**TABLE B1** True parameters of the eight scenarios with cluster size as the additional covariate.

| Scenario | $(\bar{m}, n)$ | $\beta$                    | $\gamma$                    | SACE                             | $\pi$                  |
|----------|----------------|----------------------------|-----------------------------|----------------------------------|------------------------|
| I        | (25,60)        | $[-8, -1, -0.7, -0.2]^T$   | $[-7.5, -1.4, 0.4, -0.2]^T$ | $[-7.60, -6.33, -9.38, -7.87]^T$ | $[0.1, 0.09, 0.81]^T$  |
| II       | (50,60)        |                            |                             | $[8.19, 10.17, 4.01, 6.90]^T$    |                        |
| III      | (25,60)        | $[-3.8, -1, -0.7, -0.2]^T$ | $[1.5, -1.4, 0.4, -0.2]^T$  | $[-7.26, -6.24, -9.18, -7.89]^T$ | $[0.21, 0.19, 0.60]^T$ |
| IV       | (50,60)        |                            |                             | $[7.57, 12.03, 2.06, 7.83]^T$    |                        |
| V        | (25,30)        | $[-8, -1, -0.7, -0.2]^T$   | $[-7.5, -1.4, 0.4, -0.2]^T$ | $[-7.15, -5.96, -8.88, -7.45]^T$ | $[0.1, 0.09, 0.81]^T$  |
| VI       | (50,30)        |                            |                             | $[5.43, 7.98, 1.55, 4.94]^T$     |                        |
| VII      | (25,30)        | $[-3.8, -1, -0.7, -0.2]^T$ | $[1.5, -1.4, 0.4, -0.2]^T$  | $[-7.29, -6.26, -9.16, -7.86]^T$ | $[0.21, 0.19, 0.60]^T$ |
| VIII     | (50,30)        |                            |                             | $[7.57, 12.03, 2.06, 7.83]^T$    |                        |

In all the scenarios

$$\alpha_1^{11} = \begin{bmatrix} -13 & -11 \\ -0.5 & 0.4 \\ -0.2 & 0.3 \\ 0.3 & 0.3 \end{bmatrix}, \alpha_1^{10} = \begin{bmatrix} 2 & -9 \\ 2 & -1 \\ 2 & 0.8 \\ 1 & -1 \end{bmatrix}, \alpha_0^{11} = \begin{bmatrix} 14 & 12 \\ 0.5 & 0.4 \\ -0.4 & 0.4 \\ -0.4 & -0.3 \end{bmatrix}, \Sigma_\eta = \begin{bmatrix} 1 & 0.71 \\ 0.71 & 1 \end{bmatrix}, \Sigma_e = \begin{bmatrix} 5 & 3.54 \\ 3.54 & 10 \end{bmatrix}, \phi = 1$$

**TABLE B2** Simulation results for scenario I-IV with posterior means, bias, coverage, and Monte Carlo error for ISACE, CSACE, and ICC parameters using a bivariate model or univariate outcome models with 60 clusters ( $n = 60$ ) with cluster size as a covariate in the principal stratification model. Results are average based on 100 simulations.

| Scenario | Parameter     | True value | Posterior mean | Bivariate Model |          | Monte-Carlo error | Posterior mean | Univariate Models |          | Monte-Carlo error |
|----------|---------------|------------|----------------|-----------------|----------|-------------------|----------------|-------------------|----------|-------------------|
|          |               |            |                | %Bias           | Coverage |                   |                | %Bias             | Coverage |                   |
| I        | $\delta_I^1$  | -7.60      | -7.60          | 0.08            | 0.96     | 0.10              | -6.855         | -9.88             | 0.49     | 0.16              |
|          | $\delta_I^2$  | -6.34      | -6.36          | 0.39            | 0.94     | 0.20              | -6.34          | 0.05              | 0.94     | 0.22              |
|          | $\delta_C^1$  | -9.38      | -9.35          | -0.39           | 0.96     | 0.09              | -8.63          | -8.01             | 0.54     | 0.15              |
|          | $\delta_C^2$  | -7.87      | -7.86          | -0.15           | 0.96     | 0.19              | -7.84          | -0.38             | 0.96     | 0.20              |
|          | $\rho^1$      | 0.17       | 0.17           | 0.28            | 0.98     | 0.0013            | 0.06           | -61.29            | 0.10     | 0.0005            |
|          | $\rho^2$      | 0.17       | 0.16           | 1.67            | 0.96     | 0.0013            | 0.13           | -19.47            | 0.79     | 0.0001            |
|          | $\rho_1^{12}$ | 0.08       | 0.08           | 4.60            | 0.93     | 0.0010            | —              | —                 | —        | —                 |
|          | $\rho_2^{12}$ | 0.50       | 0.50           | -0.28           | 0.96     | 0.0009            | —              | —                 | —        | —                 |
| II       | $\delta_I^1$  | 8.19       | 8.25           | 0.77            | 0.94     | 0.09              | 9.38           | 14.60             | 0.15     | 0.16              |
|          | $\delta_I^2$  | 10.17      | 10.21          | -0.31           | 0.94     | 0.18              | 10.24          | 0.66              | 0.96     | 0.24              |
|          | $\delta_C^1$  | 4.00       | 4.07           | 1.64            | 0.95     | 0.08              | 5.24           | 30.83             | 0.11     | 0.15              |
|          | $\delta_C^2$  | 6.90       | 6.93           | 0.55            | 0.93     | 0.16              | 6.95           | 0.79              | 0.98     | 0.23              |
|          | $\rho^1$      | 0.17       | 0.17           | -0.52           | 0.97     | 0.0009            | 0.05           | -72.38            | 0        | 0.0002            |
|          | $\rho^2$      | 0.17       | 0.17           | 1.2             | 0.96     | 0.0009            | 0.06           | -66.16            | 0        | 0.0003            |
|          | $\rho_1^{12}$ | 0.08       | 0.08           | -3.92           | 0.89     | 0.0007            | —              | —                 | —        | —                 |
|          | $\rho_2^{12}$ | 0.50       | 0.49           | -1.09           | 0.91     | 0.0005            | —              | —                 | —        | —                 |
| III      | $\delta_I^1$  | -7.26      | -7.35          | 1.23            | 0.91     | 0.10              | -5.48          | -24.41            | 0.11     | 0.31              |
|          | $\delta_I^2$  | -6.24      | -6.30          | 1.01            | 0.97     | 0.20              | -6.23          | -0.09             | 1        | 0.30              |
|          | $\delta_C^1$  | -9.18      | -9.19          | 0.14            | 0.97     | 0.10              | -7.44          | -18.90            | 0.09     | 0.30              |
|          | $\delta_C^2$  | -7.89      | -7.92          | 0.30            | 0.99     | 0.19              | -7.91          | 0.18              | 1        | 0.30              |
|          | $\rho^1$      | 0.17       | 0.16           | -1.95           | 0.92     | 0.0013            | 0.04           | -76.85            | 0.02     | 0.0004            |
|          | $\rho^2$      | 0.17       | 0.16           | -3.72           | 0.92     | 0.0013            | 0.07           | -59.13            | 0.10     | 0.0006            |
|          | $\rho_1^{12}$ | 0.08       | 0.08           | -7.71           | 0.94     | 0.0010            | —              | —                 | —        | —                 |
|          | $\rho_2^{12}$ | 0.50       | 0.50           | -1.12           | 0.90     | 0.0011            | —              | —                 | —        | —                 |
| IV       | $\delta_I^1$  | 7.57       | 7.57           | -0.04           | 0.97     | 0.09              | 10.26          | 35.48             | 0        | 0.39              |
|          | $\delta_I^2$  | 12.03      | 11.99          | -0.36           | 0.94     | 0.19              | 12.03          | 0.04              | 0.99     | 0.43              |
|          | $\delta_C^1$  | 2.06       | 2.06           | 0.37            | 0.96     | 0.08              | 4.85           | 135.85            | 0        | 0.39              |
|          | $\delta_C^2$  | 7.83       | 7.80           | -0.47           | 0.97     | 0.16              | 7.83           | -0.07             | 1        | 0.43              |
|          | $\rho^1$      | 0.17       | 0.16           | -1.49           | 0.92     | 0.0010            | 0.02           | -87.35            | 0        | 0.0001            |
|          | $\rho^2$      | 0.17       | 0.16           | -1.35           | 0.93     | 0.0010            | 0.02           | -84.40            | 0        | 0.0001            |
|          | $\rho_1^{12}$ | 0.08       | 0.08           | -5.62           | 0.92     | 0.0007            | —              | —                 | —        | —                 |
|          | $\rho_2^{12}$ | 0.50       | 0.50           | -0.87           | 0.91     | 0.006             | —              | —                 | —        | —                 |

**TABLE B3** Simulation results for scenario V-VIII with posterior means, bias, coverage, and Monte Carlo error for ISACE, CSACE, and ICC parameters using a bivariate model or univariate outcome models with 60 clusters ( $n = 30$ ) with cluster size as a covariate in the principal stratification model. Results are average based on 100 simulations.

| Scenario | Parameter     | Bivariate Model |                |       |          |                   | Univariate Models |        |          |                   |
|----------|---------------|-----------------|----------------|-------|----------|-------------------|-------------------|--------|----------|-------------------|
|          |               | True value      | Posterior mean | %Bias | Coverage | Monte-Carlo error | Posterior mean    | %Bias  | Coverage | Monte-Carlo error |
| V        | $\delta_I^1$  | -7.15           | -7.03          | -1.65 | 0.94     | 0.21              | -6.28             | -12.13 | 0.71     | 0.33              |
|          | $\delta_I^2$  | -5.96           | -5.85          | -1.87 | 0.95     | 0.40              | -55.86            | -1.08  | 0.98     | 0.43              |
|          | $\delta_C^1$  | -8.88           | -8.79          | -1.06 | 0.96     | 0.19              | -8.04             | -9.47  | 0.70     | 0.31              |
|          | $\delta_C^2$  | -7.45           | -7.35          | -1.33 | 0.97     | 0.37              | -7.34             | -1.49  | 0.98     | 0.40              |
|          | $\rho^1$      | 0.17            | 0.17           | 2.12  | 0.98     | 0.0027            | 0.06              | -61.56 | 0.34     | 0.0013            |
|          | $\rho^2$      | 0.17            | 0.16           | -4.15 | 0.91     | 0.0026            | 0.13              | -24.88 | 0.76     | 0.0020            |
|          | $\rho_1^{12}$ | 0.08            | 0.08           | -6.57 | 0.89     | 0.0020            | —                 | —      | —        | —                 |
|          | $\rho_2^{12}$ | 0.50            | 0.49           | -2.09 | 0.95     | 0.0020            | —                 | —      | —        | —                 |
| VI       | $\delta_I^1$  | 5.43            | 5.48           | 0.95  | 0.96     | 0.20              | 6.68              | 23.13  | 0.46     | 0.35              |
|          | $\delta_I^2$  | 7.98            | 8.02           | 0.41  | 0.95     | 0.39              | 8.07              | 1.08   | 0.97     | 0.52              |
|          | $\delta_C^1$  | 1.55            | 1.61           | 3.84  | 0.97     | 0.17              | 2.85              | 84.01  | 0.35     | 0.33              |
|          | $\delta_C^2$  | 4.94            | 4.98           | 0.87  | 0.98     | 0.35              | 5.01              | 1.42   | 1        | 0.48              |
|          | $\rho^1$      | 0.17            | 0.17           | 3.25  | 0.95     | 0.0022            | 0.05              | -71.09 | 0.08     | 0.0007            |
|          | $\rho^2$      | 0.17            | 0.17           | 1.75  | 0.95     | 0.0021            | 0.07              | -58.91 | 0.26     | 0.0009            |
|          | $\rho_1^{12}$ | 0.08            | 0.08           | -0.30 | 0.94     | 0.0017            | —                 | —      | —        | —                 |
|          | $\rho_2^{12}$ | 0.50            | 0.50           | -0.57 | 0.97     | 0.0013            | —                 | —      | —        | —                 |
| VII      | $\delta_I^1$  | -7.29           | -7.28          | -0.18 | 0.96     | 0.22              | -5.40             | -26.01 | 0.30     | 0.64              |
|          | $\delta_I^2$  | -6.26           | -6.35          | 1.54  | 0.93     | 0.41              | -6.26             | 0.08   | 0.96     | 0.60              |
|          | $\delta_C^1$  | -9.15           | -9.10          | -0.57 | 1        | 0.21              | -7.32             | -19.98 | 0.30     | 0.63              |
|          | $\delta_C^2$  | -7.86           | -7.92          | 0.70  | 0.96     | 0.39              | -7.88             | 0.32   | 0.98     | 0.59              |
|          | $\rho^1$      | 0.17            | 0.16           | -3.57 | 0.95     | 0.0029            | 0.04              | -75.16 | 0.18     | 0.0011            |
|          | $\rho^2$      | 0.17            | 0.16           | -6.10 | 0.93     | 0.0029            | 0.07              | -59.26 | 0.52     | 0.0015            |
|          | $\rho_1^{12}$ | 0.08            | 0.07           | -9.60 | 0.91     | 0.0022            | —                 | —      | —        | —                 |
|          | $\rho_2^{12}$ | 0.50            | 0.49           | -2.69 | 0.98     | 0.0025            | —                 | —      | —        | —                 |
| VIII     | $\delta_I^1$  | 8.11            | 8.10           | -0.04 | 0.90     | 0.19              | 10.88             | 34.22  | 0.07     | 0.80              |
|          | $\delta_I^2$  | 12.43           | 12.53          | 0.82  | 0.93     | 0.39              | 12.59             | 1.29   | 1        | 0.87              |
|          | $\delta_C^1$  | 2.94            | 2.93           | -0.29 | 0.95     | 0.17              | 5.79              | 97.13  | 0.05     | 0.80              |
|          | $\delta_C^2$  | 8.49            | 8.59           | 1.25  | 0.92     | 0.34              | 8.61              | 1.43   | 1        | 0.85              |
|          | $\rho^1$      | 0.17            | 0.17           | 0.18  | 0.96     | 0.0021            | 0.02              | -88.11 | 0.01     | 0.0003            |
|          | $\rho^2$      | 0.17            | 0.17           | 1.20  | 0.93     | 0.0022            | 0.03              | -83.49 | 0.01     | 0.0003            |
|          | $\rho_1^{12}$ | 0.08            | 0.08           | -4.09 | 0.93     | 0.0017            | —                 | —      | —        | —                 |
|          | $\rho_2^{12}$ | 0.50            | 0.49           | -1.07 | 0.94     | 0.0013            | —                 | —      | —        | —                 |

## APPENDIX C: BOXPLOTS FOR GEWEKE DIAGNOSTIC P-VALUES FOR ICCS AND REGRESSION COEFFICIENTS

**FIGURE C1** Boxplots for Geweke diagnostic p-values of ICCs and regression coefficients for bivariate joint model Senario I-IV

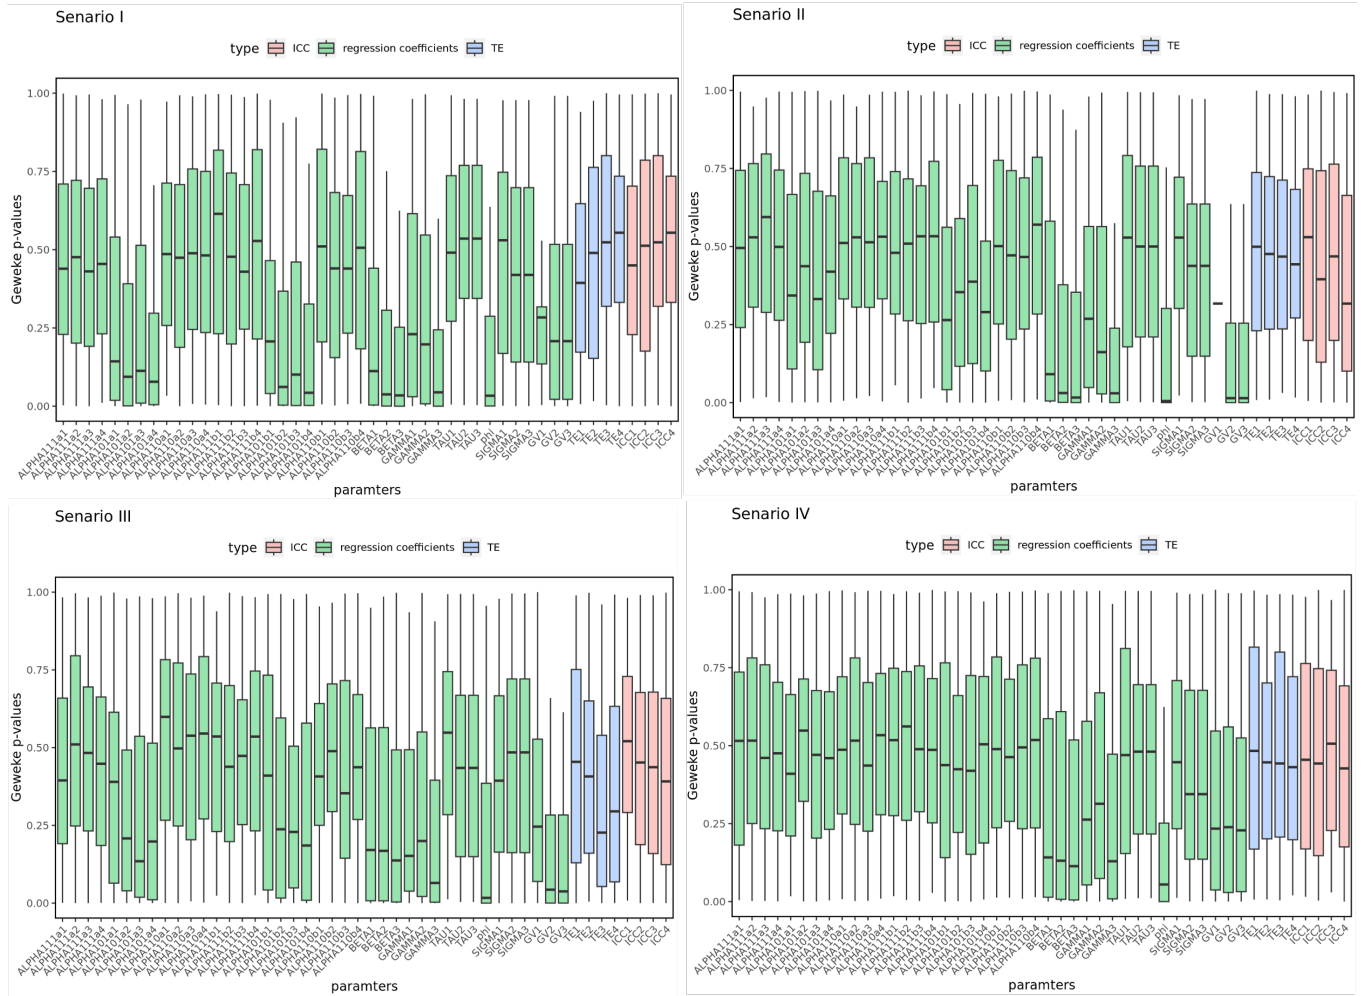

**FIGURE C2** Boxplots for Geweke diagnostic p-values of ICCs and regression coefficients for bivariate joint model Senario V-VIII

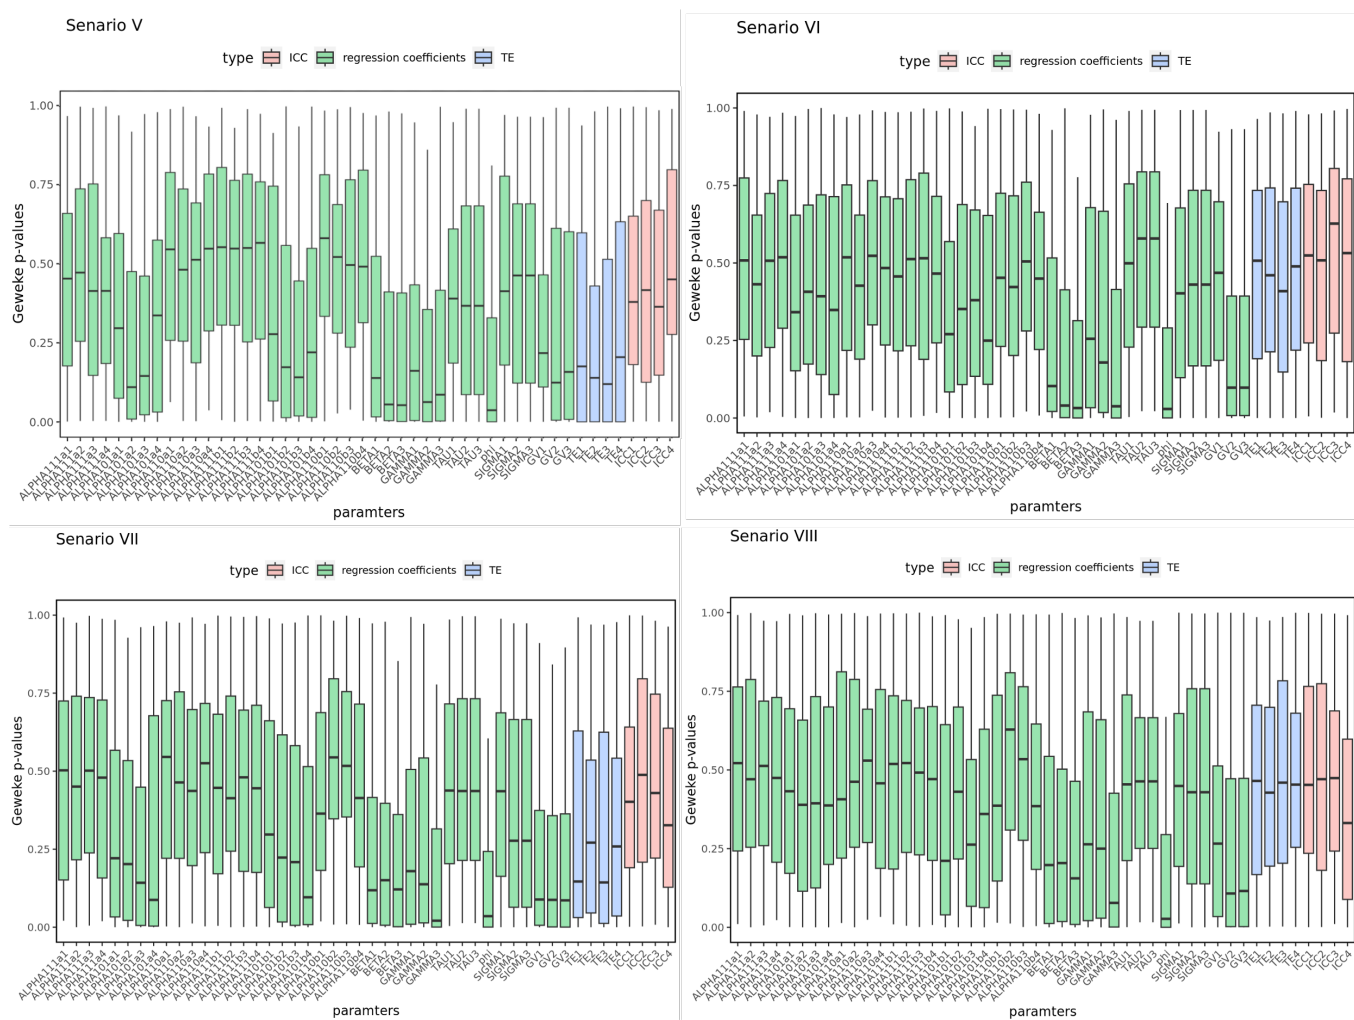

**FIGURE C3** Boxplots for Geweke diagnostic p-values of ICCs and regression coefficients for bivariate joint model with cluster size as a covariate in the principal stratification model Senario I-IV

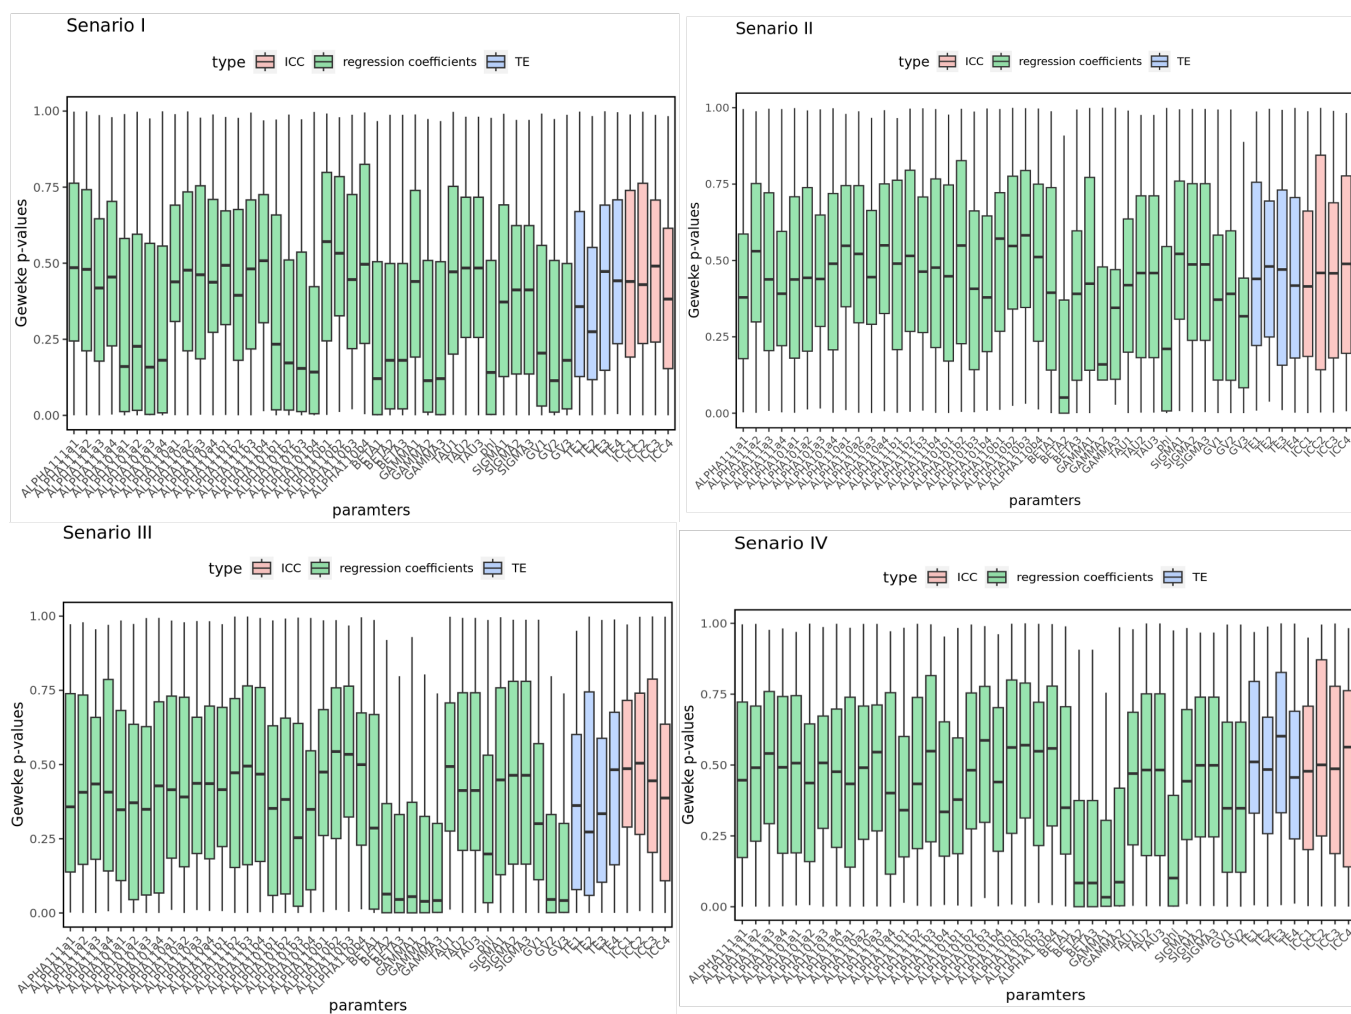

**FIGURE C4** Boxplots for Geweke diagnostic p-values of ICCs and regression coefficients for bivariate joint model with cluster size as a covariate in the principal stratification model Senario V-VIII

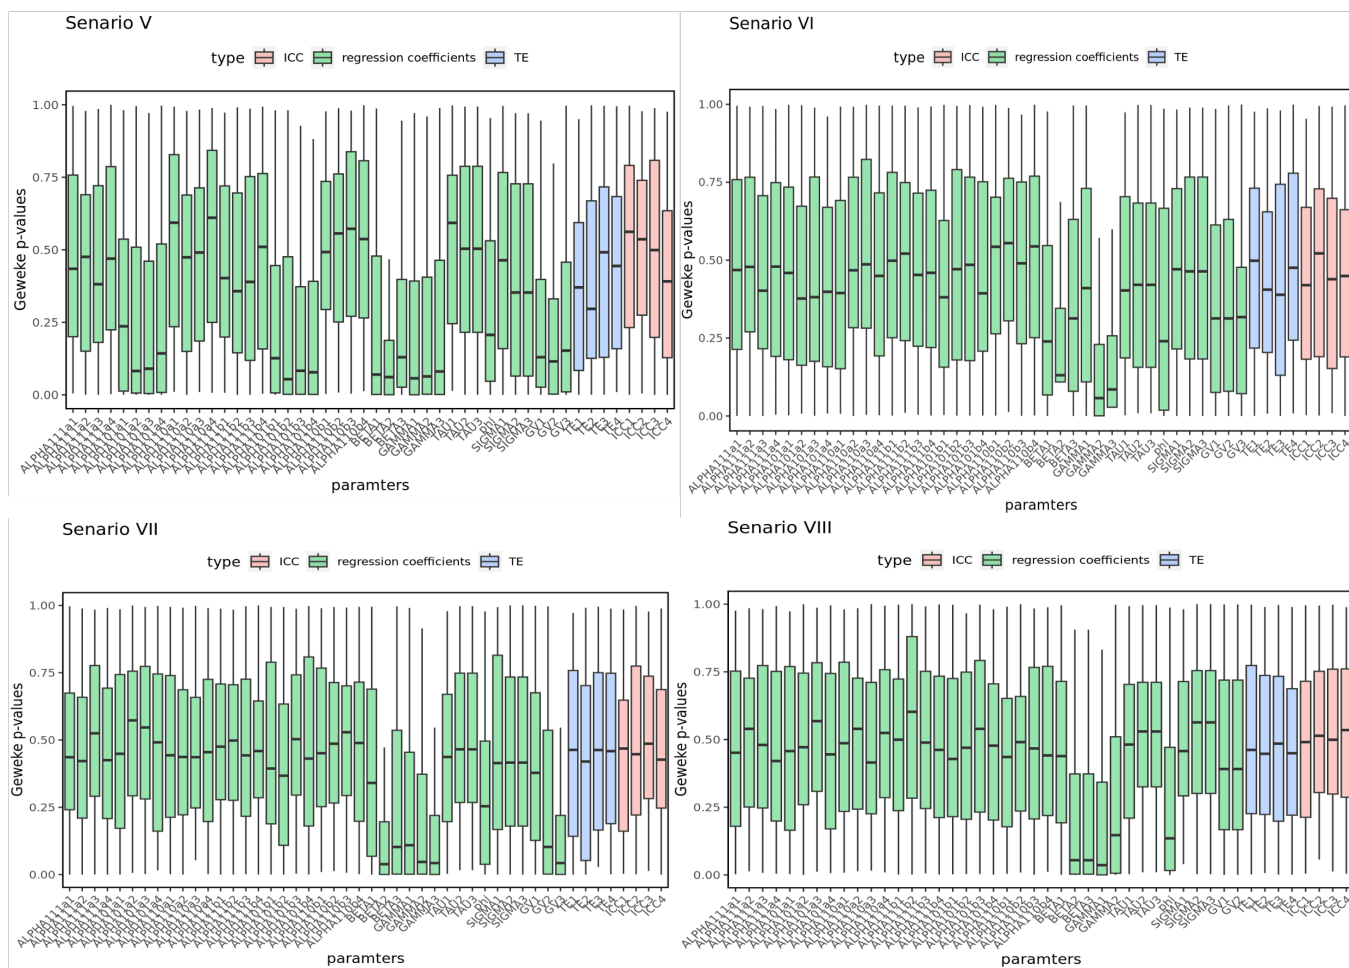

## APPENDIX D: SENSITIVITY ANALYSIS OF VIOLATING NESTED MAR ASSUMPTION

**TABLE D1** Simulation results for scenario V-VIII under the violation of nested missing at random (NMAR) with posterior means, bias, coverage, and Monte Carlo error for ISACE, CSACE, and ICC parameters using a bivariate model with 30 clusters ( $n = 30$ ). Pseudo  $R^2$  for the two level of missingness are 0.85 and 0.40 respectively. Results are average based on 100 simulations.

| Scenario | Parameter        | True value | Posterior mean | %Bias  | Coverage | Monte-Carlo error |
|----------|------------------|------------|----------------|--------|----------|-------------------|
| V        | $\delta_I^1$     | -8.46      | -8.86          | 4.83   | 0.88     | 0.29              |
|          | $\delta_I^2$     | -7.18      | -7.41          | 3.12   | 0.93     | 0.48              |
|          | $\delta_C^1$     | -10.00     | -10.72         | 7.35   | 1        | 0.29              |
|          | $\delta_C^2$     | -8.50      | -9.00          | 5.47   | 0.99     | 0.47              |
|          | $\rho^1$         | 0.17       | 0.16           | -5.00  | 0.90     | 0.0029            |
|          | $\rho^2$         | 0.17       | 0.16           | -6.03  | 0.94     | 0.0029            |
|          | $\rho_{12}^{12}$ | 0.08       | 0.07           | -12.98 | 0.85     | 0.0022            |
|          | $\rho_2^{12}$    | 0.50       | 0.49           | -1.89  | 0.94     | 0.0021            |
| VI       | $\delta_I^1$     | 11.23      | 11.37          | 2.07   | 0.92     | 0.20              |
|          | $\delta_I^2$     | 9.69       | 9.77           | 1.22   | 0.94     | 0.36              |
|          | $\delta_C^1$     | 8.04       | 7.95           | -1.14  | 0.97     | 0.19              |
|          | $\delta_C^2$     | 6.96       | 6.84           | -1.63  | 0.99     | 0.34              |
|          | $\rho^1$         | 0.17       | 0.17           | 1.51   | 0.96     | 0.0021            |
|          | $\rho^2$         | 0.17       | 0.16           | -3.36  | 0.96     | 0.0020            |
|          | $\rho_{12}^{12}$ | 0.08       | 0.08           | -4.45  | 0.92     | 0.0016            |
|          | $\rho_2^{12}$    | 0.50       | 0.49           | -1.46  | 0.92     | 0.0013            |
| VII      | $\delta_I^1$     | -8.54      | -8.94          | 4.68   | 0.85     | 0.26              |
|          | $\delta_I^2$     | -7.37      | -7.64          | 3.74   | 0.94     | 0.50              |
|          | $\delta_C^1$     | -10.13     | -11.05         | 9.15   | 1        | 0.24              |
|          | $\delta_C^2$     | -8.74      | -9.45          | 8.15   | 0.99     | 0.47              |
|          | $\rho^1$         | 0.17       | 0.17           | 2.09   | 0.94     | 0.0035            |
|          | $\rho^2$         | 0.17       | 0.16           | -5.94  | 0.90     | 0.0035            |
|          | $\rho_{12}^{12}$ | 0.08       | 0.08           | -4.77  | 0.95     | 0.0027            |
|          | $\rho_2^{12}$    | 0.50       | 0.49           | -2.13  | 0.97     | 0.0028            |
| VIII     | $\delta_I^1$     | 13.46      | 13.42          | -0.73  | 0.91     | 0.20              |
|          | $\delta_I^2$     | 11.49      | 11.41          | -1.01  | 0.98     | 0.39              |
|          | $\delta_C^1$     | 10.13      | 9.85           | -4.16  | 1        | 0.18              |
|          | $\delta_C^2$     | 8.62       | 8.38           | -3.95  | 1        | 0.36              |
|          | $\rho^1$         | 0.17       | 0.18           | 7.06   | 0.97     | 0.0023            |
|          | $\rho^2$         | 0.17       | 0.16           | -5.25  | 0.97     | 0.0022            |
|          | $\rho_{12}^{12}$ | 0.08       | 0.08           | -0.26  | 0.98     | 0.0017            |
|          | $\rho_2^{12}$    | 0.50       | 0.48           | -4.56  | 0.89     | 0.0019            |
